# Supplementary material for: Orthogonal Random Forest for Causal Inference
Source: arXiv:1806.03467 source file (2019-09-25)
Supplement: Supplementary file 1 [file old_appendix_main_theorems.tex]

\section{OLD STUFF}
\vsedit{\begin{lemma}[Uniformly Bounding
    $\Lambda(\theta)$]\label{lem:lambda-n} For any $x$:
\begin{equation}
\Ex{}{\sup_{\theta \in \Theta} \|\Lambda(\theta)\|_{\infty}} = {O}\left( s^{-\tau} +
    \psimax\sqrt{\frac{s\ln(n)}{n}}\right) 
\end{equation}
\end{lemma}}

\begin{proof}[Proof sketch of \Cref{lem:lambda-n}]
  We will rewrite the expression of $\Lambda(\theta)$ by adding and
  subtracting the term $\mu(\theta) = \Ex{}{\Psi(\theta)}$, where the
  expectation is taken over both the random draws of the observations
  and the internal randomness of the algorithm. By leveraging the
  honesty property of the kernel weights, we can rewrite $\mu(\theta)$
  as the following.
\begin{lemma}\label{exp-proof}
  For any $\theta$,
  $$\mu(\theta) = \Ex{}{\sum_{i: Z_i \in D_2} a_{i}\,
    m(x_i; \theta,\hat h)}.$$
\end{lemma}


Then we can decompose $\Lambda(\theta)$ as a sum of two error terms
such that the first one is \emph{kernel error} due to the kernel
averaging around a neighborhood of $x$, and the second one is
\emph{sampling error} due to the sampling error of the moment:
\begin{align*}
  &\Lambda(\theta)  =~  m(x; {\theta}, \hat{h}) - \mu({\theta}) +  \mu({\theta}) - \Psi(\theta)\\
  &  = \underbrace{\Ex{}{\sum_{i: Z_i \in D_2} a_{i}\cdot \left(m(x; {\theta}, \hat{h}) - m(x_i; {\theta}, \hat{h})\right)}}_{\Gamma(\theta)=\text{kernel error}}
    \\ & + \underbrace{\mu(\theta) - \frac{1}{B} \sum_{b=1}^B \sum_{i:Z_i \in D_2} a_{ib} \cdot \psi(Z_i; {\theta}, \hat{h})}_{\Delta(\theta)=\text{sampling error}}
\end{align*}

By the assumption of kernel shrinkage and the Lipschitzness of the $m$
in the first input $x$, we can bound the kernel error by
$O(s^{-\tau})$. To bound the sampling error, first observe that
$\sum_{i: Z_i\in D_2} a_{ib}\cdot \psi_j(Z_i; {\theta}, \hat{h})$ is
computed based on a random sub-sample of $D_2$ (without replacement),
and thus each coordinate $\Psi_j(\theta)$ can be viewed as a Monte
Carlo approximation to a $U$-statistic, centered at
$\mu_j(\theta)$. Hence, we can bound the sampling error with high
probability using concentration inequality. Finally, to uniformly
bound the sampling error for all $\theta$, we will apply union bound
over an $\eps$-cover over the set $\Theta$, for sufficiently small
value of $\eps$.
\end{proof}


\begin{proof}[proof of \Cref{thm:converge}]
  By \Cref{lem:lambda-n}, we have
  $\Lambda(\hat \theta) \leq \sqrt{p} \, {O}\left( s^{-\tau} +
    \psimax\sqrt{\frac{s \, p\, \ln(p\, n/ s)}{n}}\right) \equiv E$.
  Since $\hat \theta$ is consistent (proof deferred in the appendix),
  the second term $\|\hat\theta - \theta_0(x)\|^2$ is at most
  $\frac{1}{2}\|\hat{\theta} - \theta_0(x)\|$. Further, since the
  nuisance estimation error term is in smaller order than
  $E/\sqrt{p}$, we can bound $\|\hat{\theta} - \theta_0(x)\| \leq E$,
  as desired.
\end{proof}




\subsection{Proof of Asymptotic Normality}\label{app:normality}

We will show asymptotic normality of $\hat{\alpha}=\ldot{\beta}{\hat{\theta}}$ for some arbitrary direction $\beta \in \reals^p$, with $\|\beta\|_2\leq R$. Consider the complete multi-dimensional $U$-statistic:
\begin{equation}
    \Psi_0(x; \theta) = \binom{n}{s}^{-1} \sum_{S_b \subset [n]: |S_b|=s} \sum_{i\in S_b}\alpha_{S_b}(X_i) \psi(Z_i; \theta) \,.
\end{equation}
Define $\tilde{\theta} = \theta(x) - M_0^{-1} \Psi_0(x;\theta(x))$ and let
\begin{equation}
\tilde{\alpha} \triangleq \ldot{\beta}{\tilde{\theta}} = \ldot{\beta}{\theta(x)} - \ldot{\beta}{M_0^{-1}\, \Psi_0(x; \theta(x))} 
\end{equation}
For shorthand notation let $\alpha_0=\ldot{\beta}{\theta(x)}$, $\psi_\beta(Z; \theta) = \ldot{\beta}{M_0^{-1} \psi(Z;\theta)}$ and 
\begin{equation}
\Psi_{0,\beta}(x;\theta) = \ldot{\beta}{M_0^{-1}\, \Psi_0(x; \theta(x))} = \binom{n}{s}^{-1} \sum_{S_b \subset [n]: |S_b|=s} \sum_{i\in S_b}\alpha_{S_b}(X_i) \psi_{\beta}(Z_i; \theta)
\end{equation}
be a single dimensional complete $U$-statistic. Thus we can re-write:
\begin{align*}
    \tilde{\alpha} = \alpha_0 - \Psi_{0,\beta}(x;\theta(x))
\end{align*}
We then have the following lemma which its proof is provided in Appendix \ref{app:hajek}:
\begin{lemma}\label{lem:normality_of_U}
Under the conditions of Theorem \ref{thm:normality}:
\begin{equation*}
    \frac{\Psi_{0,\beta}(x;\theta(x))}{\sigma_n(x)} \rightarrow N(0,1)\,,
\end{equation*}
for $\sigma_n^2(x) = \frac{s^2}{n}\Var\bb{\E\bb{\sum_{i=1}^sK(x, X_i, \{X_j\}_{j=1}^s) \psi_{\beta}(Z_i; \theta)\mid X_1}} = \Omega(\frac{s^2}{n} \eta(s))$.
\end{lemma}
Invoking Lemma~\ref{lem:normality_of_U} and using our assumptions on the kernel, we conclude that:
\begin{equation}
    \frac{\tilde{\alpha} - \alpha_0(x)}{\sigma_n(x)} \rightarrow \normal(0,1).
\end{equation}
For some sequence $\sigma_n^2$ which decays at least as slow as $s^2 \eta(s)/n$.
Hence, since 
\[
\frac{\hat{\alpha}-\alpha_0}{\sigma_n(x)} = \frac{\tilde{\alpha}-\theta(x)}{\sigma_n(x)} + \frac{\hat{\alpha}-\tilde{\alpha}}{\sigma_n(x)},
\]
if we show that $\frac{\hat{\alpha}-\tilde{\alpha}}{\sigma_n(x)}\rightarrow_p 0$, then by Slutsky's theorem we also have that: 
\begin{equation}
    \frac{\hat{\alpha}-\alpha_0}{\sigma_n(x)} \rightarrow \normal(0,1),
\end{equation}
as desired. Thus, it suffices to show that:
\begin{equation}
    \frac{\|\hat{\alpha} - \tilde{\alpha}\|_2}{\sigma_n(x)} \rightarrow_p 0.
\end{equation}
Observe that since $\|\beta\|_2 \leq R$, we have $\|\hat{\alpha} - \tilde{\alpha}\|_2\leq R \|\hat{\theta} - \tilde{\theta}\|_2$. Thus it suffices to show that:
\begin{equation*}
 \frac{\|\hat{\theta} - \tilde{\theta}\|}{\sigma_n(x)} \rightarrow_p 0.
\end{equation*}
\begin{lemma}\label{lem:remainder_normality}
Under the conditions of Theorem~\ref{thm:normality}, for $\sigma_n^2(x)= \Omega\bp{\frac{s^2}{n} \eta(s)}$:
\begin{equation}\label{eqn:htheta-acc}
 \frac{\|\hat{\theta} - \tilde{\theta}\|}{\sigma_n(x)} \rightarrow_p 0.
\end{equation}
\end{lemma}
\begin{proof}
Performing a second-order Taylor expansion of $m_j(x; \theta)$ around $\theta(x)$ and observing that $m_j(x;\theta(x))=0$, we have that for some $\bar{\theta}_j\in\Theta$:
\begin{align*}
    m_j(x;\hat{\theta}) =~& \ldot{\nabla_{\theta} m_j(x;\theta(x))}{\hat{\theta} - \theta(x)} +  \underbrace{(\hat{\theta}-\theta(x))^\top H_j(x;\bar{\theta}_j) (\hat{\theta}-\theta(x))^\top}_{\rho_j}\,.
\end{align*}
Letting $\rho=(\rho_1,\ldots, \rho_p)$, writing the latter set of equalities for each $j$ in matrix form, multiplying both sides by $M_0^{-1}$ and re-arranging, we get that:
\begin{equation*}
 \hat{\theta}  = \theta(x) + M_0^{-1} m (x;\hat{\theta})  - M_0^{-1}\rho \,.
\end{equation*}
Thus by the definition of $\tilde{\theta}$ we have:
\begin{equation*}
    \hat{\theta}-\tilde{\theta} = M_0^{-1} \cdot (m(x;\hat{\theta}) + \Psi_0(x;\theta(x))) - M_0^{-1}\rho \,.
\end{equation*}
By the bounds on the eigenvalues of $H_j(x;\theta)$ and $M_0^{-1}$, we have that:
\begin{equation}
    \|M_0^{-1}\rho\|_2 \leq \frac{L_H}{\lambda} \|\hat{\theta}-\theta(x)\|_2^2 \,.
\end{equation}
Thus we have:
\begin{equation*}
    \|\hat{\theta}-\tilde{\theta}\|_2 = \frac{1}{\lambda} \|m(x;\hat{\theta}) + \Psi_0(x;\theta(x))\|_2 +\frac{L_H}{\lambda} \|\hat{\theta}-\theta(x)\|_2^2 \,.
\end{equation*}

We now argue about the convergence rate of the first term on the right hand side. Similar to the proof of Theorem \ref{thm:mse_rate}, since $\Psi(x;\hat{\theta})=0$ we have:
\begin{align*}
   m(x;\hat{\theta}) = m(x; \hat{\theta}) - \Psi(x; \hat{\theta})
   = m(x; \hat{\theta}) - \Psi_0(x; \hat{\theta}) + \underbrace{\Psi_0(x; \hat{\theta}) - \Psi(x;\hat{\theta})}_{\text{subsampling error}} \,.
\end{align*}
Let $\mu_0(x;\theta) = \E\bb{\Psi_0(x;\theta)}$, which due to honesty and similar to Lemma \ref{lem:mu-eq}, we have: 
\[
\mu_0(x;\theta) = \sum_{i=1}^n \E \bb{\alpha(X_i) m(X_i,\theta)}.
\]
Thus we can add and subtract $\mu_0$ from $m(x;\hat{\theta})$ as:
\begin{align*}
   m(x;\hat{\theta}) =~& \underbrace{m(x; \hat{\theta}) - \mu_0(x;\hat{\theta})}_{C=\text{Kernel error}} + \underbrace{\mu_0(x; \hat{\theta}) - \Psi_0(x; \hat{\theta})}_{D=\text{Sampling error}} + \underbrace{\Psi_0(x; \hat{\theta}) - \Psi(x;\hat{\theta})}_{E=\text{Subsampling error}}\,.
\end{align*}
Now similar to proof of Theorem \ref{thm:mse_rate} we bound different terms separately and combine the results.
\paragraph{Kernel Error.} Term $C$ is a kernel error and hence is upper bounded by $\epsilon(s)$ in expectation. Since, by assumption $s$ is chosen such that $\epsilon(s)=o(\sigma_n(x))$, we ge that $\|C\|_2/\sigma_n(x)\rightarrow_p 0$. 

\paragraph{Subsampling Error.}
Term $E$ is a sub-sampling error, which can be made arbitrarily small if the number of drawn sub-samples is large enough and hence $\|E\|_2/\sigma_n(x)\rightarrow_p 0$. In fact, similar to the part about bounding subsampling error in Lemma \ref{lem:lambda_bound_mse} we have that that:
\begin{equation*}
    \E_{S_b}\bb{\sum_{i\in S_b} \alpha_{S_b}(X_i) \psi(Z_i;\theta)} = \Psi_0(x;\theta)\,,
\end{equation*}
Therefore, $\Psi(x;\theta)$ can be thought as the sum of $B$ independent random variables each with expectation equal to $\Psi_0(x;\theta)$. Now we can invoke Corollary \ref{cor:bracketing} in the appendix for the trivial U-process, with $s=1, n=B$ to get that with probability $1-\delta_1$:
\begin{equation*}
    \sup_{\theta \in \Theta} \| \Psi_0(x;\theta)-\Psi(x;\theta)\| \leq O \bp{\Psi_{\max} \sqrt{\frac{\log\log(B)+\log(1/\delta_1)}{B}}}\,.
\end{equation*}
Hence, for $B\geq (n/s)^{5/4}$, due to our assumption that $\bp{s/n \log\log(n/s)}^{5/8} = o(\sigma_n(x))$ we get $\|E\|_2/\sigma_n(x)\rightarrow_p 0$.

\paragraph{Sampling Error.} We focus on term $D$ now. By adding and subtracting $\Psi_0(x;\theta(x))$ we have:
\begin{align*}
    D =~& \mu_0(x; \hat{\theta}) + \Psi_0(x;\theta_0) - \Psi_0(x; \hat{\theta}) - \Psi_0(x;\theta(x))\,.
\end{align*}
Further adding and subtracting $\mu_0(x;\theta(x))$, as well as subtracting $m(x;\theta(x))$, which is zero by definition of $\theta(x)$, we have:
\begin{align*}
    D =~& \underbrace{\mu_0(x; \hat{\theta})-\mu_0(x; \theta(x)) + \Psi_0(x;\theta(x)) - \Psi_0(x; \hat{\theta})}_{F=\text{Stochastic equicontinuity term}} + \underbrace{\mu_0(x;\theta(x)) - m(x;\theta(x))}_{G=\text{Kernel error}} - \Psi_0(x;\theta(x)) \,.
\end{align*}
Term $G$ is a kernel error term and hence is upper bounded in expectation by the kernel shrinkage rate of $\epsilon(s)$, which by a similar argument as term $C$, satisfies that $\|G\|_2/\sigma_n(x) \rightarrow 0$. 

Thus it suffices that show that $\|F\|_2/\sigma_n(x)\rightarrow_p 0$, in order to conclude that $\frac{\|m(x;\hat{\theta}) + \Psi_0(x;\theta(x))\|_2}{\sigma_n(x)}\rightarrow_p 0$.
Term $D$ can be re-written as:
\begin{equation}
    F = \Psi_0(x;\theta(x)) - \Psi_0(x; \hat{\theta}) - \E\bb{\Psi_0(x;\theta(x)) - \Psi_0(x; \hat{\theta})}\,.
\end{equation}
Observe that each coordinate $j$ of $F$, is a stochastic equicontinuity term for $U$-processes over the class of symmetric functions $\text{conv}(\cF_j)=\{f_j(\cdot;\theta): \theta \in \Theta\}$, with $f_j(Z_1,\ldots, Z_{s};\theta) = \sum_{i=1}^{s} \alpha_{Z_{1:s}}(X_i) (\psi_j(Z_i; \theta(x))-\psi_j(Z_i;\theta))$. Observe that since $f_j\in \text{conv}(\cF_j)$ is a convex combination of functions in $\cF_j=\{\psi_j(\cdot; \theta(x))-\psi_j(\cdot;\theta): \theta \in \Theta\}$, the bracketing number of functions in $\text{conv}(\cF_j)$ is upper bounded by the bracketing number of $\cF_j$, which in turn is upper bounded by the bracketing number of the function class $\{\psi_j(\cdot;\theta): \theta \in \Theta\}$, which by our assumption, satisfies $\log(N_{[]}({\cal F}_j, \epsilon, L_2))= O(1 /\epsilon)$. 
Moreover, under the variogram assumption and the lipschitz moment assumption we have that if $\|\theta-\theta(x)\|\leq r\leq 1$, then:
\begin{align*}
     \|f_j(\cdot;\theta)\|_{P,2}^2  =~& \E\bb{\bp{\sum_{i=1}^{s} \alpha_{Z_{1:s}}(X_i) (\psi_j(Z_i; \theta(x))-\psi_j(Z_i;\theta)}^2}\\
     \leq~& \E\bb{\sum_{i=1}^{s} \alpha_{Z_{1:s}}(X_i) \bp{\psi_j(Z_i; \theta(x))-\psi_j(Z_i;\theta)}^2} \tag{Jensen's inequality}\\
     =~& \E\bb{\sum_{i=1}^{s} \alpha_{Z_{1:s}}(X_i) \E\bb{\psi_j(Z_i; \theta(x))-\psi_j(Z_i;\theta)}^2|X_i]} \tag{honesty of kernel}\\
     =~&\E\bb{\sum_{i=1}^{s} \alpha_{Z_{1:s}}(X_i) \left(\Var(\psi(Z;\theta(x)) - \psi(Z;\theta)|X_i)  + \left(m(X_i;\theta(x)) - m(X_i;\theta)\right)^2\right)}\\
    \leq~& L_\psi \|\theta-\theta(x)\| + L_J^2 \|\theta - \theta(x)\|^2 \leq L_\psi r + L_J^2 r^2 = O(r)\,.
\end{align*}
Moreover, $\|f_j\|_{\infty}\leq 2\psi_{\max}$. Thus we can apply Corollary~\ref{cor:bracketing}, with $\eta= \sqrt{L_\psi r + L_J^2 r^2}=O(\sqrt{r})$ and $G=2\psi_{\max}$ to get that if $\|\hat{\theta}-\theta(x)\|\leq r$, then w.p. $1-\delta/p$:
\begin{align*}
    |F_j| \leq~& \sup_{\theta: \|\theta-\theta(x)\|\leq r} \left|\Psi_0(x;\theta(x)) - \Psi_0(x; \hat{\theta}) - \E\bb{\Psi_0(x;\theta(x)) - \Psi_0(x; \hat{\theta})}\right|\\
    =~& O\left( \left(r^{1/4} + \sqrt{r} \sqrt{\log(p/\delta) + \log\log(n/(s\,r))}\right) \sqrt{\frac{s}{n}}\right)\\
    =~& O\left( \left(r^{1/4}\sqrt{\log(p/\delta) + \log\log(n/s)}\right) \sqrt{\frac{s}{n}}\right)\triangleq \kappa(r,s,n,\delta)\,.
\end{align*}
Using a union bound this implies that with probability $1-\delta$ we have
\begin{equation*}
    \max_j |F_j| \leq \kappa(r,s,n,\delta)\,.
\end{equation*}
By our MSE theorem and also Markov's inequality, with probability $1-\delta'$: $\|\hat{\theta}-\theta(x)\|\leq \nu(s)/\delta'$, where:
\[
\nu(s) = \frac{1}{\lambda}\left(L_m \epsilon(s) + O\left(\psi_{\max}\sqrt{\frac{p\, s}{n} \log\log(p\, s /n)}\right)\right)
\]
Thus using a union bound with probability $1-\delta-\delta'$, we have:
\begin{align*}
    \max_j |F_j| = O\left(\kappa(\nu(s)/\delta', s, n, \delta))\right)\,
\end{align*}
To improve readability from here we ignore all the constants in our analysis, while we keep all terms (even $\log$ or $\log\log$ terms) that depend on $s$ and $n$. Note that we can even ignore $\delta$ and $\delta'$, because they can go to zero at very slow rate such that terms $\log(1/\delta)$ or even $\delta'^{1/4}$ appearing in the analysis grow slower than $\log\log$ terms. Now, by the definition of $\nu(s)$ and $\kappa(r, s, n, \delta')$, as well as invoking the inequality $(a+b)^{1/4} \leq a^{1/4} + b^{1/4}$ for $a,b >0$ we have:
\begin{equation}
    \max_j |F_j| \leq O(\kappa(\nu(s)/\delta', s, n, \delta)) \leq O\left(\epsilon(s)^{1/4} \left(\frac{s}{n}\log\log(n/s)\right)^{1/2} + \left(\frac{s}{n}\log\log(n/s)\right)^{5/8}\right)\,,
\end{equation}
Hence, using our Assumption on the rates in the statement of Theorem \ref{thm:normality} we get that both of the terms above are $o(\sigma_n(x))$. Therefore, $\|F\|_2/\sigma_n(x) \rightarrow_p 0$. Thus, combining all of the above, we get that:
\begin{equation*}
    \frac{\|\tilde{\theta}-\hat{\theta}\|}{\sigma_n(x)} = o_p(1)
\end{equation*}
as desired.
\end{proof}



\section{Missing Proofs in \Cref{GMM}}



\vsedit{
\begin{proof}[Proof of~\Cref{lem:taylor}]
  Fix a conditioning vector $x$. By performing a second order Taylor expansion of each coordinate $j\in [p]$ of the expected score
  function around the true parameters $\theta_0=\theta_0(x)$ and $h_0$ and
  applying the multi-dimensional mean-value theorem, we can write
  \begin{align*}
 m_j(x; \theta, \hat h) &= m_j(x; \theta_0, h_0) + \nabla_\theta  m_j(x; \theta_0, h_0)' (\theta - \theta_0) + D_{\psi_j}[\hat h - h_0 \mid x]\\
    &+ \underbrace{\Ex{}{((\theta, \hat{h}(W)) - (\theta_0, h_0(W)))^\intercal\nabla^2_{\theta, h} \psi_j(Z; \tilde{\theta}_j, \tilde{h}_j(W)) ((\theta, \hat{h}(W)) - (\theta_0, h_0(W))\mid x}}_{\rho_j}
  \end{align*}
  where each $\tilde \theta_j$ is some convex combination of $\theta$
  and $\theta_0$ and each $\tilde h_j(W)$ is some convex combination of
  $\hat h(W)$ and $h_0(W)$.  
  Note that $m(x; \theta_0, h_0) = 0$ by definition and
$D_{\psi_j}[\hat h - h_0 \mid x] = 0$ by local orthogonality.  Let $\rho$ denote the vector of second order terms. We can thus write the above set of equations in matrix form as:
\begin{equation*}
M  (\theta - \theta_0)  = m(x; \theta, \hat h) - \rho
\end{equation*}
where we remind that 
$M=\nabla_\theta m(x; \theta_0, h_0)$ is the Jacobian of the moment vector. Since by our assumptions $M$ is invertible
and has eigenvalues bounded away from zero by a constant, we can write:
\[
  ({\theta} - \theta_0) = M^{-1}\, m(x;\theta, \hat h) + M^{-1}\, \rho
\]
By the boundedness of the eigenvalues of $M^{-1}$, we thus have:
\begin{equation*}
\|\theta - \theta_0\| = O(\|m(x; \theta, \hat h)\|) + O\left(\sqrt{p}\, \|\rho\|_{\infty}\right)
\end{equation*}
By our bounded eigenvalue Hessian assumption, we know that:
\[
  \|\rho\|_{\infty} = O\left( \Ex{}{\|\hat h(W) - h_0(W) \|^2\mid x} + \|
  \theta - \theta_0\|^2 \right)
\]
Combining the above two equations recovers our claim.
\end{proof}
}

\begin{proof}[Proof of \Cref{exp-proof}]
  Consider any example $Z_i\in D_2$ and iteration $b\in [B]$.  We will
  write $\xi$ to denote the internal randomness of the algorithm, and
  write $Z_{-i}$ to denote the random draws of all of the examples in
  $D$ other than $Z_i$. For any realized feature vector $x_i$, we know
  the weight $a_{ib}$ is a deterministic function of $Z_{-i}, x_i$ and
  $\xi$. \swcomment{todo: udpate honesty} At the same time, we have for any estimate $\hat h$,
  \[
    \Ex{}{\psi(Z_i; \theta, \hat h(W_i))\mid Z_{-i}, x_i, \xi} =
    \Ex{}{\psi(Z_i; \theta, \hat h(W_i))\mid x_i} = m(x_i; \theta,
    \hat h)
  \]
 Thus, we can write:
  \begin{align*}
\Ex{}{a_{ib} \, \psi(Z_i; \theta, \hat h(W_i)) \mid x_i , \hat h } &= \Ex{Z_{-i}, \xi\mid  x_i , \hat h }{\Ex{}{a_{ib} \, \psi(Z_i; \theta, \hat h(W_i))\mid Z_{-i}, x_i, \hat h, \xi}}\\
    &= \Ex{Z_{-i}, \xi\mid  x_i , \hat h }{\Ex{}{a_{ib} \mid Z_{-i}, x_i, \hat h, \xi} \Ex{}{ \psi(Z_i; \theta, \hat h(W_i))\mid Z_{-i},  x_i, \hat h, \xi}}\\
    &=\Ex{Z_{-i}, \xi\mid  x_i , \hat h }{\Ex{}{a_{ib} \mid Z_{-i}, x_i, \hat h, \xi} m(x_i; \theta, \hat h)}\\
    &=\Ex{Z_{-i}, \xi\mid  x_i , \hat h}{\Ex{}{a_{ib} \, m(x_i; \theta, \hat h)\mid Z_{-i}, x_i, \hat h, \xi} } =   \Ex{}{a_{ib} \, m(Z_i; \theta, \hat h) \mid x_i , \hat h }
  \end{align*}
  By the law of iterated expectation, we also get
  \begin{align*}
   \Ex{}{a_{ib} \cdot \psi(Z_i; \theta, \hat h(W_i))} &= \Ex{x_i, \hat h}{\Ex{}{a_{ib} \, \psi(Z_i; \theta, \hat h(W_i)) \mid x_i , \hat h}}
                                                         % &= \Ex{x_i, \hat h, i\in S_b^3}{\Ex{}{a_{ib} \, m(Z_i; \theta, \hat h) \mid x_i , \hat h , i \in S_b^3}}\\
    = \Ex{x_i, \hat h}{\Ex{}{a_{ib} \, m(Z_i; \theta, \hat h) \mid x_i , \hat h}} = \Ex{}{a_{ib} \, m(Z_i; \theta, \hat h)}
% &= \Ex{x_i , \hat h}{\Ex{}{a_{ib} \cdot \psi(Z_i; \theta, \hat
                                                         %   h(W_i))\mid  x_i, \hat h }}\\
                                                         % &= \Ex{x_i , \hat h}{{\Ex{}{a_{ib} \mid  x_i, \hat h} \, \Ex{}{ \psi(Z_i; \theta, \hat
                                                         %   h(W_i))\mid  x_i, \hat h}}}\\
                                                         % &= \Ex{x_i , \hat h}{{\Ex{}{a_{ib} \mid Z_i \in S_b^3,
                                                         %   x_i, \hat h} \, { m(x_i; \theta, \hat h)}}}\\
                                                         % &= \Ex{x_i , \hat h}{{\Ex{}{a_{ib}  m(x_i; \theta, \hat h)\mid Z_i \in S_b^3,
                                                         %   x_i, \hat h} \, }} \\ &= \Ex{}{a_{ib}\,  m(x_i; \theta, \hat h)\mid Z_i \in S_b^3} 
  \end{align*}
By linearity of expectation, we can then rewrite $\mu(\theta)$ as follows:
\begin{align*}
  \mu({\theta}) =
                    &\frac{1}{B}\sum_{b=1}^B \sum_{i: Z_i\in D_2}   \Ex{}{a_{ib} \,  m(x_i; \theta, \hat h)} 
\end{align*}
This completes the proof.
 \end{proof}



% \subsection{Proof of \Cref{superman}}\label{sec:sampled-u-stat}







\begin{proof}[Proof of \Cref{lem:lambda-n}]
The first step is to rewrite the expression of $\Lambda_n(\theta)$ by
adding and subtracting the term $\mu(\theta)$. 
This allows us to
decompose $\Lambda_n(\theta)$ as a sum of two error terms such that
the first one is due to the kernel averaging around a neighborhood of
$x$, and the second one is due to the sampling error of the moment at
every data point. Formally, for any
$\theta$, 

\begin{align*}
  &\Lambda_n(\theta)  =~  m(x; {\theta}, \hat{h}) - \mu({\theta}) +  \mu({\theta}) - \frac{1}{B}\sum_{b=1}^B\sum_{i: Z_i\in D_2} a_{ib} \cdot \psi(Z_i; {\theta}, \hat{h})\\
  &  = \frac{1}{B}\underbrace{\Ex{}{\sum_{b=1}^B\sum_{i: Z_i \in D_2} a_{ib}\cdot \left(m(x; {\theta}, \hat{h}) - m(x_i; {\theta}, \hat{h})\right)}}_{\Gamma(\theta)=\text{kernel error}}
    +  \underbrace{\mu(\theta) - \frac{1}{B}\sum_{b=1}^B\sum_{i:Z_i \in D_2} a_{ib} \cdot \psi(Z_i; {\theta}, \hat{h})}_{\Delta(\theta)=\text{sampling error}}
\end{align*}



\paragraph{Bounding kernel error via shrinkage.} The Kernel error
$\Gamma$ is bounded by the Lipschitzness of the conditional moment
function and the kernel shrinkage assumption:
\vsedit{
\begin{align*}
\Ex{}{\sup_{\theta \in \Theta} \left\|  \Gamma(\theta) \right\|_{\infty}} \leq~& \Ex{}{\sup_{\theta \in \Theta} \frac{1}{B}\sum_{b=1}^B\sum_{i: Z_i \in D_2} a_{ib}\cdot \left\| m(x; {\theta}, \hat{h}) - m(x_i; {\theta}, \hat{h}) \right\|_{\infty}}\\
  \leq~& L\cdot \Ex{}{\frac{1}{B}\sum_{b=1}^B \sum_{i: Z_i\in D_2} a_{ib}\cdot \|x-x_i\|_2}\\
  \leq~& L\frac{1}{B}\sum_{b=1}^B  \Ex{}{\sup \{\|x-x_i\|_2: a_{ib}>0\}}   \leq {\cal O}\left(s^{-\tau}\right)
\end{align*}
}
where the first inequality follows from triangle inequality, second
follows from Lipschitzness of $m$, third follows from the form of the
normalization of kernel weighting function, and the last follows from
the kernel shrinkage assumption.




\paragraph{Bounding sampling error via $U$-statistics.} 
Fix any nuisance estimate $\hat h$, then each term
$\sum_{i: Z_i\in D_2} a_{ib}\cdot \psi_j(Z_i; {\theta}, \hat{h})$ is
computed based on a random sub-sample of $D_2$ (without replacement)
in the input data set $S$. In particular, it can be viewed as a Monte
Carlo approximation to a U-statistics. By the concentration of
U-statistic and standard Chernoff bound~\cite{Hoeffding}, we can
obtain the following tail bound on $\Psi(\theta, \hat h)$. (See the
appendix for proofs.)

\begin{lemma}\label{superman}
  Fix any estimate $\theta$, moment coordinate $j\in [p]$ and  $\delta \in (0, 1)$. Then with probability at least
  $1 - \delta$ over the randomness of the random draws of $D$ and the
  internal randomness of the algorithm,
\vsedit{  
\[
  \left| \Delta_j(\theta) \right| =  \left|\Psi_j(\theta, \hat h) - \mu_j(\theta) \right| \leq
    \mathcal{O}\left(\psimax\sqrt{\ln(1/\delta)\left(
          {\frac{s}{n}}\right) } \right)
  \]
  }
  as long as $B \geq n/s$ and $|\psi_j(Z; \theta, \hat h)|\leq \psimax$
  for any $\theta\in \Theta$ and observation $Z$.
\end{lemma}

To prove \Cref{superman}, let us derive a high-probability bound for
the sampling error term $\Delta(\theta)$ in the decomposition of
$\Lambda_n$. First, consider the following base function $f_0$ defined
in \Cref{alg:basefunction} that is parameterized by a base kernel
learner $\cL_k$, a target point $x$ and estimate $\theta$.

\begin{algorithm}
\begin{algorithmic}
  \STATE{\textbf{Input}: data set $S$ of size $s$}
  \STATE{\textbf{Initialize}: For each $z_i\in S$, set weight
    $a_{ib} = 0$ for all $b\in[B]$}
  \INDSTATE{Let $S^1$, $S^2$, and $S^3$ denote the first,
    second, and third $s/3$ parts of the input data set $S$}

    \INDSTATE{Let $K$ be the kernel function computed by $\cL_k$
      using data set $S^1$}

    \INDSTATE{Let $H = \{z \in S^2\mid K(x, x_i, S^2) > 0\}$ be
      the set of points with non-zero weight}

    \INDSTATE{Compute nuisance estimator $\hat h$ using the data set
      $H$}
    
    \STATE{\textbf{Output}:
    $\sum_{z_i \in S^3} K(x, x_i, S^3) \psi(z_i; \theta, \hat h)$}
   
  \caption{Base function $f_0$, parameterized by a target point $x$,
    an estimate $\theta$, and a base kernel learner
    $\cL_k$} \label{alg:basefunction}

\end{algorithmic}
\end{algorithm}


Given this definition of base function, we will also define the
following function $f_\theta$ that takes as input $s$ number of examples:
\[
  f_\theta(z_1, \ldots , z_s) = \frac{1}{s!} \sum_{p} f_0(z_1', \ldots ,
  z_s')
\]
where $\sum_p$ denotes the summation over all of the $s!$ number of
permutations $(z_1', \ldots, z_s')$ of the input examples
$(z_1, \ldots, z_s)$. Finally, given a dataset $D$ of $n$ observations
and any fixed integer $s$, we condider the following U-statistic:
\[
  U_\theta(D) = \frac{1}{{n\choose s}} \sum_{c} f_\theta(z_{i1}, \ldots , z_{is})
\]
where $\sum_c$ denotes the summation over all of the ${n \choose s}$
combinations of $s$ distinct choices in $D$. 

Observe that we can view $U_\theta(D)$ as a random variable with randomness
taken over the random draws of $D$. Then its expectation satisfies
\[
\Ex{D}{U_\theta(D)} = \mu(\theta).
\]

The following first-order tail inequality for U-Statistics is useful
for our analysis.

\begin{theorem}[\cite{Hoeffding}]\label{hoeffding-u}
  For any $\eps > 0$,
  \[
    \Pr_{D}\left[ |U_\theta(D) - \mu(\theta)| \geq \eps \right] \leq
    2\exp\left( - (n/s)\eps^2\right)
  \]
  Equivalently, for any $\delta \in (0, 1)$, with probability
  $1 - \delta$,
  $ \left| U_\theta(D) - \mu(\theta) \right| \leq \sqrt{\frac{1}{n/s}
    \ln(2/\delta)}$. 
\end{theorem}
\iffalse
have for any fixed $\theta$ and any $\eta > 0$,
\begin{equation}\label{concentration}
  \Pr\left[\left|\frac{1}{B}\sum_{b=1}^B\sum_{i=1}^n a_{ib} \cdot \psi(z_i; \theta, \hat h_b) - \mu(\theta)\right| \geq \xi\right] \leq 2\exp\left\{- \frac{n}{s} {\xi^2}\right\}
\end{equation}
\fi


\noindent Recall that
  $$\Psi(\theta, \hat h) = \frac{1}{B} \sum_{b=1}^B \sum_{i=1}^n
  a_{ib} \psi(z_i; \theta, \hat h_b)$$ We can obtain a
  high-probability bound for the deviation between
  $\Psi(\theta, \hat h)$ and $U_\theta(D)$ for any fixed data set $D$.


\begin{lemma}\label{chernoff-psi}
  Fix any $\theta\in \Theta$, data set $D$ and number of iterations
  $B$. Then with probability at least
  $1 - \delta$ over the randomness of the algorithm,
  \[
    |\Psi(\theta, \hat h) - U_\theta(D)| \leq \sqrt{\frac{\ln(2/\delta)}{2B}}
  \]
\end{lemma}


\begin{proof}
  Note that in each iteration $b$ of the algorithm, the quantity
  $\sum_{i=1}^n a_{ib}\psi(z_i; \theta, \hat h_b)$ satisfies
\[
  \Ex{}{\sum_{i=1}^n a_{ib}\psi(z_i; \theta, \hat h_b)} = U_\theta(D)
\]
Then we can view $\Psi(\theta, \hat h)$ as the average of $B$
i.i.d. random variables with mean $U_\theta(D)$. By applying the standard
Chernoff bound \sw{cite}, we have for any $\eps > 0$,
\[
  \Pr\left[\left|\Psi( \theta, \hat h) - U_\theta(D) \right| > \eps\right]
  \leq 2\exp\left( {-2B\eps^2}\right)
\]
Then setting the deviation $\eps = \sqrt{\ln(2/\delta)/(2B)}$ recovers
our stated bound.
\end{proof}


\paragraph{Proof of \Cref{superman}}By combining the results from
\Cref{hoeffding-u} and \Cref{chernoff-psi}, we can also bound the
difference between $\Psi(\theta, \hat h)$ and $\mu(\theta)$.  The
final bound follows from the fact that $\sqrt{s/n} \succeq \sqrt{1/B}$
as long as $B\geq n/s$.




Next, we will use a covering number argument to bound
\[
  \Ex{}{ \sup_{\theta\in \Theta} \left\|\Psi(\theta, \hat h) - \mu(\theta)\right\|_{\infty}}
\]




\noindent Let $\cC = \cC(\Theta, \eps)$ be $\eps$-cover over the set
$\Theta$, that is, for any $\theta\in \Theta$, there exists some
$\theta' \in \cC$ such that $\|\theta - \theta'\|_2\leq \eps$. Observe, that when $\Theta$ 
is a bounded set in $\RR^p$ with constant diameter, then by standard arguments, there exists a 
cover of size $1/\epsilon^p$.


\vsedit{
\begin{proof}
  Let $\cC(\Theta, \eps)$ be a cover of $\Theta$, of size $O(1/\epsilon^p)$, which is guaranteed to exist by the boundedness of $\Theta$. By applying the concentration bound in \Cref{superman} and a union
  bound over all $\theta \in \cC(\Theta, \eps)$ and $j\in [p]$, we have with
  probability at least $1 - \delta$ that
\[
  \sup_{\theta\in \cC} \left\|\Psi(\theta, \hat h) - \mu(\theta)\right\|_{\infty}
 =
  {\cal O}\left( \psimax \sqrt{\frac{s \ln(|\cC|\, p/\delta)}{n}} \right) = {\cal O}\left( \psimax \sqrt{\frac{s \, p\, \ln(p/ (\epsilon\, \delta))}{n}} \right)
\]
Then 
by the Lipchtizness of $\psi$ in $\theta$ for any $\hat h$ and $Z_i$ and also the boundedness of $\psi$, we also have
\[
  \Ex{}{ \sup_{\theta\in \Theta} \left\|\Psi(\theta, \hat h) -
      \mu(\theta)\right\|_{\infty}} = {\cal O}\left( \psimax \sqrt{\frac{s\, p\, 
        \ln(p/(\eps\delta))}{n}} + \eps + \delta \psimax \right)
\]
Setting the parameters $\eps \leq O(\sqrt{s/n})$ and
$\delta \leq O(\sqrt{s/n})$, we can obtain the stated bound.
% $\Ex{}{|\Delta(\hat \theta)|} = {\cal O}\left(\frac{\ln(
%     n/s)}{\sqrt{n/s}}\right)$.
\end{proof}
}

\vsedit{\begin{lemma}\label{highprob}
  Fix any nuisance estimate $\hat h$ from the first stage such that
  $\|\psi(Z; \theta, \hat h)\|_{\infty}\leq \psimax$ for any $\theta\in \Theta$
  and observation $Z$. Then
  \begin{align*}
   \Ex{}{ \sup_{\theta\in \Theta} \left\|\Delta(\theta)\right\|_{\infty}} =  \Ex{}{ \sup_{\theta\in \Theta} \left\|\Psi(\theta, \hat h) - \mu(\theta)\right\|_{\infty}}\\
    \leq {O}\left(\psimax\sqrt{\frac{s\, p\, \ln(p\, n/s)}{n}} \right)
  \end{align*}
\end{lemma}
}

Combining our bounds on $\Gamma(\theta)$ and $\Delta(\theta)$ yields the proof of Lemma~\ref{lem:lambda-n}.
\end{proof}


\vsedit{\subsection{Consistency}
The latter proof assumes consistency of $\hat{\theta}$ so as to argue that the quadratic term $\|\hat{\theta}-\theta_0\|_2^2$ is negligible for $n$ large enough. It remains to show that $\hat{\theta}$ is also consistent to conclude the proof. We first provide a simple proof of consistency that simply adds the extra assumptions of a strictly unique solution to the moment equation and also Lipschitzness of the expected moment equation with respect to both parameters. This proof does not yield an explicit preliminary rate, but is asymptotic. In the next section we provide a setting under which we can argue consistency at an explicit preliminary rate, which is more desirable for finite sample performance.
\begin{lemma}
Suppose that:
\begin{enumerate}
\item $\theta_0(x)$ is the unique solution to $m(x; \theta, h_0)=0$, i.e. $\forall \epsilon > 0: \inf\{ \|m(x; \theta, h_0)\|: \|\theta - \theta_0(x)\| \geq \epsilon\} > 0$
\item The moment $m(x; \theta, h)$ is $L$-Lipschitz continuous in $\theta$ w.r.t. $\|\cdot\|$ and also continuous in $h$ w.r.t. the $L^1$ norm $\|f\|=\Ex{}{\|f(W)\| \mid x}$ for every $\theta, h$ and $x$.
\item The first stage estimate is consistent w.r.t. the $L^2$ norm: $\sqrt{\Ex{}{\|\hat h(W) - h_0(W) \|^2\mid x}} = O_p(h_n) = o_p(1)$
\item The subsampling level $s$ is chosen such that $\epsilon_n =  {O}\left( s^{-\tau} +    \psimax\sqrt{\frac{s\ln(n)}{n}}\right) = o(1)$
\end{enumerate}
Then the estimate $\hat{\theta}$ is consistent for $\theta_0(x)$, i.e. $\|\hat{\theta}-\theta_0(x)\| = o_p(1)$.
\end{lemma}
\begin{proof}
By Lemma \ref{lem:lambda-n} and our assumption on the setting of $s$, we have that $\|m(x; \hat{\theta}, \hat{h})\| = \|\Lambda_n(\hat{\theta})\| = o_p(1)$. Since $m(x; \theta, h)$ is Lipschitz in $h$ and $\hat{h}$ is consistent at a rate $h_n$ w.r.t to the $L^2$ and hence also $L^1$ norm, we have: $\|m(x; \hat{\theta}, h_0)\| = \|m(x; \hat{\theta}, \hat{h})\| + O_p(h_n) = o_p(1)$. By our first assumption, for any $\epsilon$, there exists a $\delta$, such that: $\Pr[\|\hat{\theta}-\theta_0(x)\| \geq \epsilon] \leq \Pr[\|m(x; \hat{\theta}, h_0)\|\geq \delta]$. Since $\|m(x; \hat{\theta}, h_0)\| = o_p(1)$, the probability on the right-hand-side converges to $0$ and hence also the left hand side. Hence, $\|\hat{\theta}-\theta_0(x)\| = o_p(1)$.
\end{proof}
}

\subsubsection{Consistency for Gradients of Convex Losses}
\vsedit{ We show that the latter is true if the moment $\psi$ is the sub-gradient of a convex loss function $\ell$, i.e. $\psi(Z; \theta, h(W)) = \partial_\theta \ell(Z; \theta, h(W))$, moreover, we require that gradient of $m(x; \theta, h)$ with respect to $\theta$ is Lipschitz in $h$.
\begin{lemma}[Consistency under Convexity] Suppose that:
\begin{enumerate}
\item The moment $\psi$ is the gradient of a convex loss $\ell$, i.e. $\psi(Z; \theta, h(W)) = \nabla_\theta \ell(Z; \theta, h(W))$.
\item The eigenvalues of the Jacobian $\nabla_\theta m(x; \theta, h_0)$ are lower bounded by $\sigma>0$ for every $\theta$ and $x$. Every entry of the Jacobian $\nabla_\theta m(x; \theta, h)$  is $L$-Lipschitz in $h$ w.r.t. the $L^1$ norm $\|f\|=\Ex{}{\|f(W)\| \mid x}$ for every $\theta$ and $x$.
\item The first stage estimate is consistent w.r.t. the $L^2$ norm: $\sqrt{\Ex{}{\|\hat h(W) - h_0(W) \|^2\mid x}} = O_p(h_n) = o_p(1)$
\item The subsampling level $s$ is chosen such that $\epsilon_n =  {O}\left( s^{-\tau} +    \psimax\sqrt{\frac{s\ln(n)}{n}}\right) = o(1)$
\end{enumerate}
Then the estimate $\hat{\theta}$ is consistent for $\theta_0(x)$ at a rate $O_p(\frac{2}{\sigma - O_p(L h_n p)}\sqrt{p} (\epsilon_n + h_n^2))$.
\end{lemma}
\begin{proof}
Since the Jacobian of the expected moment $m(x; \theta, h_0)$ has eigenvalues lower bounded by $\sigma$ and each entry of the Jacobian of $\psi$ is $L$-Lispchitz with respect to the nuisance, we have that for every vector $\nu \in \RR^p$ (with $p$ the dimension of $\theta(x)$):
\begin{align*}
\frac{\nu^T \nabla_{\theta} m(x; \theta, \hat{h}) \nu}{\|\nu\|^2} \geq~& \frac{\nu^T \nabla_{\theta} m(x;\theta, h_0) \nu}{\|\nu\|^2} + \frac{\nu^T \left(\nabla_{\theta} m(x; \theta, \hat{h}) - m(x;\theta, h_0)\right) \nu}{\|\nu\|^2} \geq \sigma - L\cdot \Ex{}{\|\hat{h}(W) - h_0(W) \| \mid x} \frac{\|\nu\|_1^2}{\|\nu\|_2^2}\\
\geq~& \sigma - O_p(L\, h_n\, p) = \sigma - o_p(1)
\end{align*}
Where in the last inequality we also used Holder's inequality to upper bound the $L^1$ norm by the $L^2$ norm of the first stage error. Thus the expected loss function $L(\theta) = \Ex{}{\ell(Z; \theta, \hat{h}(W) \mid x}$ is $\hat{\sigma} = \sigma - o_p(1)$ strongly convex, since $\nabla_{\theta} m (x; \theta, \hat{h})$ is the Hessian of $L(\theta)$. We then have:
\begin{align*}
L(\hat{\theta}) - L(\theta_0) \geq \nabla_{\theta} L(\theta_0)' (\hat{\theta} - \theta_0) + \frac{\hat{\sigma}}{2} \|\hat{\theta}-\theta_0\|_2^2 =  m(x; \theta_0, \hat{h})' (\hat{\theta}-\theta_0) + \frac{\hat{\sigma}}{2} \|\hat{\theta}-\theta_0\|_2^2
\end{align*}
Moreover, by convexity of $L(\theta)$, we have:
\begin{align*}
L(\theta_0) - L(\hat{\theta}) \geq \nabla_\theta L(\hat{\theta})' ( \theta_0 - \hat{\theta}) = m(x; \hat{\theta}, \hat{h})' ( \theta_0 - \hat{\theta})
\end{align*}
Combining the above we get:
\begin{align*}
\frac{\hat{\sigma}}{2} \|\hat{\theta}-\theta_0\|_2^2 \leq (m(x; \hat{\theta}, \hat{h}) - m(x; \theta_0, \hat{h}) )' ( \hat{\theta}- \theta_0 ) \leq \| m(x; \hat{\theta}, \hat{h}) - m(x; \theta_0, \hat{h})\|_2\, \|  \hat{\theta}- \theta_0 \|_2
\end{align*}
Dividing over by $\|\hat{\theta}-\theta_0\|$, we get:
\begin{align*}
\|\hat{\theta}-\theta_0\|_2 \leq \frac{2}{\hat{\sigma}} \left( \| m(x; \hat{\theta}, \hat{h})\|_2 + \| m(x; \theta_0, \hat{h})\|_2\right)
\end{align*}
The term $\| m(x; \hat{\theta}, \hat{h})\|_2$ is upper bounded by $\|\Lambda_n(\hat{\theta})\|_2$, which was shown in Lemma \ref{lem:lambda-n} to be of order:  ${O}\left( \sqrt{p} \left(s^{-\tau} + \psimax\sqrt{\frac{s\ln(n)}{n}}\right)\right)=o(1)$. Subsequently, using a second order Taylor expansion around $h_0$ and orthogonality argument almost identical to the proof of Lemma \ref{lem:taylor}, we can show that the second term $\|m(x; \theta_0, \hat{h})\|_2$ is it upper bounded by $O_p(\sqrt{p}\, h_n^2)=o_p(1)$. Hence, $\|\hat{\theta}-\theta_0\|_2 = o_p(1)$, which completes the proof of consistency.
\end{proof}
}
